# Supplementary material for: Training independent subnetworks for robust prediction
Source: arXiv:2010.06610 source file (2021-08-04)
Supplement: Supplementary file 1 [file appendix.tex]

Through this training procedure, we are able to train $M$ subnetworks that operate independently. We make three claims that we support with empirical evidence. First, that outputs are invariant w.r.t. the inputs not corresponding to them, second, the outputs exhibit the same diversity as independently trained neural networks and third, the $M$ subnetworks use disjoint parts of the network.

In our analysis, we examine the diversity between predictive distributions. Specifically, we look at three distance metrics:
\begin{enumerate}
    \item Disagreement: The probability that the predicted class differs in a classification task. $\mathrm{D}_{\text{disagreement}}(P_1, P_2) = \mathrm{I}(\argmax_{\hat{y}} P_1(\hat{y}) = \argmax_{\hat{y}} P_2(\hat{y}))$. The disagreement between identical predictive distributions is 0.
    \item Kullback–Leibler divergence: $\KL(p_1, p_2) = \E_{p_1}\left[\log p_1(y) - \log p_2(y) \right]$. The KL-divergence between identical predictive distributions is 0.
    \item Cosine similarity: The cosine similarity of the predicted class probabilities in a classification task. $\mathrm{D}_{\text{cosine}}(P_1, P_2) = \frac{\sum_{\hat{y}} P_1(\hat{y})P_2(\hat{y}) }{\sqrt{\sum_{\hat{y}}P_1(\hat{y})^2 }\sqrt{\sum_{\hat{y}}P_2(\hat{y})^2 }}$. The cosine similarity between identical predictive distributions is 1.
\end{enumerate}

\paragraph{Invariance} We claim that in the trained model, the outputs are invariant to the inputs not corresponding to them. In the case of $M=3$, this means that $p_\theta(\rvy_1|\rvx_1, \rvx_2, \rvx_3)\approx p_\theta(\rvy_1|\rvx_1, \rvx'_2, \rvx'_3)$ where $(\rvx_1, \rvy_1), (\rvx_2, \rvy_2), (\rvx_3, \rvy_3), (\rvx'_2, \rvy'_2), (\rvx'_3, \rvy'_3) \in \sX$. Note that invariance holds in the empirical sense not in the mathematical sense. Invariance is learnt by the network as a result of the inputs being independently sampled from the training set, hence only the corresponding input carrying useful information for each output. To measure invariance, we examine the diversity in the predictions as the inputs vary:
\begin{equation}
    \mathcal{I}_{\mathrm{D}}=\E\left[\mathrm{D}\left(p_\theta(\rvy_1|\rvx_1, \rvx_2 \dots \rvx_M), p_\theta(\rvy_1|\rvx_1, \rvx'_2 \dots \dots \rvx'_M)\right) \right] \,,
\end{equation}
where $\mathrm{D}$ is a distance metric between predictive distributions and $(\rvx_1, \rvy_1) \dots (\rvx_M, \rvy_M), (\rvx'_2, \rvy'_2) \dots (\rvx'_M, \rvy'_M) \in \sX$. We only analyse the first input-output pair $(\rvx_1, \rvy_1)$ since all the pairs behave similarly due to symmetry. We find that the input-output pair is close to invariant on both the training and test sets as shown in Table \ref{tab:invariance}.
% $\mathcal{I}_{\mathrm{D}_{\text{disagreement}}}=0.016996, $\mathcal{I}_{\KL}=0.022616 $\mathcal{I}_{\mathrm{D}_{\text{cosine}}}=0.99275 % Test
% $\mathcal{I}_{\mathrm{D}_{\text{disagreement}}}=0.00000$, $\mathcal{I}_{\KL}=0.000656$ $\mathcal{I}_{\mathrm{D}_{\text{cosine}}}=1.00000$ % Train
\begin{table}[h!]
    \centering
\begin{tabular}{lccc}
\hline
                  &   {$\mathcal{I}_{\mathrm{D}_{\text{disagreement}}}$} &   {$\mathcal{I}_{\KL}$} &   {$\mathcal{I}_{\mathrm{D}_{\text{cosine}}}$} \\
\hline
 MIMO (size=3)          &                      0.000 / 0.017      &               0.001 / 0.023    &             1.000 / 0.99275     
 \\
 \hline
\end{tabular} 
    \caption{The invariance of the first input-output pair w.r.t. the other inputs. The metrics show that predictions are only slightly affected the other inputs. ResNet28-10, Cifar10 Training / Test sets. }
    \label{tab:invariance}
\end{table}
